# Supplementary material for: On the Equivalency, Substitutability, and Flexibility of Synthetic Data
Source: arXiv:2403.16244 source file (2024-03-24)
Supplement: Supplementary file 1 [file __supplemental.tex]

% \noindent We organize the Supplementary Materials as follows:

% %%%%%%%%%%%%%% Genarator
% \noindent \textbf{A. Data Generator: {\datagenerator}}

% \quad \textbf{A.1. Authoring of Group Activities in {\datagenerator}}

% \quad \textbf{A.2 List of Variables for Domain Randomization}

% %%%%%%%%%%%%%% Experiments
% \noindent \textbf{B. More Details of Experiments}

% \quad \textbf{B.1 2D Skeleton-based Group Activity Recognition}

% \quad \textbf{B.2 RGB-based Multi-Person Pose Tracking}

% \quad \textbf{B.3 3D Group Activity Generation}

% %%%%%%%%%%%%%% Dataset
% \noindent \textbf{C. Dataset Details and Comparisons}

% % \quad \textbf{C.1 \texttt{{\datagenerator}2D}}

% % \quad \textbf{C.2 \texttt{{\datagenerator}RGB}}

% % \quad \textbf{C.3 \texttt{{\datagenerator}3D}}

% %%%%%%%%%%%%%% Dataset
% \noindent \textbf{D. Discussions on Limitations and Future Work}

% \bigskip
% \bigskip

This document provides more details about our data generator, datasets, and experiments. 
We also include additional results to supplement the main text. 
In addition to this supplementary material, all the data, code, videos, tools and related materials are organized at \href{http://cjerry1243.github.io/M3Act}{http://cjerry1243.github.io/M3Act}.

%%%%%%%%%%%%%% Genarator
\section*{A. Data Generator: {\datagenerator}}
\subsection*{A.1. Authoring of Group Activities}
Authoring group activities in {\datagenerator} is non-trivial because people adhere to social norms while forming groups.
% of the different semantics of group activities. 
The authoring requires nuanced adjustments varied from group to group, including the alignment of characters, their orientations, and the permitted atomic actions.
We summarize these rules and adjustments in Tab.~\ref{tab:authoring_groups}. 
For example, characters in a talking group are positioned in a circle facing the center. 
For queueing groups, characters can form a straight line, curve, etc., and individuals in a queue can be texting, idling, talking, and so on.

Group walking, running (jogging), and dancing are the three group activities with drastic body movements.
Particularly, collision avoidance is one social norm that is implicitly followed by humans during collective walking or running. Therefore,  we propose a simple algorithm to dynamically adjust the animation speed for each character engaged in the walking and running activities, thus mitigating avatar collisions. 
The detailed algorithm is shown in Alg.~\ref{alg:collision_avoidance}. 
Specifically, the animation speed of a character decreases when any character is in front of it and close to it. 
When no potential collision is detected, the animation speed of a character can increase up to its initial speed.
While animating complex interactions for group dancing is challenging, we enforce nearly synchronous movements for all individuals.
\begin{table*}[]
\setlength{\tabcolsep}{8.6pt}
% \small
\footnotesize
% \scriptsize
% \fontsize{9.5pt}{9.5pt}\selectfont
  \aboverulesep=0ex
  \belowrulesep=0ex 
%   \vspace{6pt}
\begin{center}
\setlength{\tabcolsep}{5.6pt}
\begin{tabular}{c|c|c|c|c}
\toprule
\textbf{Activity Name} & \textbf{Alignment} & \textbf{Face At} & \textbf{Atomic Actions} & \textbf{Other Conditions} \\
\midrule \midrule
\multirow{2}{*}{Walking} & \multirow{2}{*}{Straight Line, Circle, Rectangle} & \multirow{2}{*}{Same Direction} & \multirow{2}{*}{walk} &  \multirow{2}{*}{Adjust animation speed at runtime} \\
 & & & & \\
\hline
\multirow{2}{*}{Waiting} & \multirow{2}{*}{Multi-Row Straight Lines} & \multirow{2}{*}{Same Direction} & \multirow{2}{*}{idle, text, talk, point, wave} & \multirow{2}{*}{N/A} \\
 & & & & \\

\hline

\multirow{2}{*}{Queueing} & \multirow{1}{*}{Straight Line, One-Corner Line,} & \multirow{2}{*}{Front of Queue} & \multirow{2}{*}{idle, text, talk, point} & \multirow{2}{*}{N/A} \\
 & Two-Corner Line, Parabola, Curve & & & \\
\hline

\multirow{2}{*}{Talking} & \multirow{2}{*}{Circle} & \multirow{2}{*}{Group Center} & \multirow{2}{*}{talk} & \multirow{2}{*}{N/A} \\
 & & & & \\
\hline

\multirow{2}{*}{Dancing} & \multirow{2}{*}{Multi-Row Straight Lines} & \multirow{2}{*}{Same Direction} & \multirow{2}{*}{dance} & \multirow{2}{*}{Nearly-synchronous movements}  \\
& & & & \\

\hline

\multirow{2}{*}{Jogging} & \multirow{2}{*}{Straight Line, Circle, Rectangle} & \multirow{2}{*}{Same Direction} & \multirow{2}{*}{run} & \multirow{2}{*}{Adjust animation speed at runtime} \\
 & & & & \\
\bottomrule
\end{tabular}
\end{center}
\vspace{-10pt}
\caption{Rules and adjustments for activity authoring.}
\label{tab:authoring_groups}
\end{table*}

\begin{table*}[]
\setlength{\tabcolsep}{6.6pt}
% \small
\footnotesize
% \scriptsize
% \fontsize{9.5pt}{9.5pt}\selectfont
  \aboverulesep=0ex
  \belowrulesep=0ex 
%   \vspace{6pt}
\begin{center}
\setlength{\tabcolsep}{5.6pt}
\begin{tabular}{c|c|c|c}
\toprule
\textbf{Category} & \textbf{Randomizer} & \textbf{Variable} & \textbf{Distribution} \\
\midrule
\midrule
\multirow{2}{*}{Scenes} & Scene Selection  & scene & a set of prebuilt 3D environments \\
\cline{2-4}
 & HDRI Selection & hdri & a set of collected HDRIs
 \\

\midrule
\multirow{4}{*}{Camera} & \multirow{4}{*}{Camera Position } & radius & Uniform(6, 10) \\
 &  & camera rotation & Uniform(0, 360) \\
 &  & camera height & Uniform(1, 5) \\
 &  & perturbation & Cartesian[Uniform(-1, 1), 0 Uniform(-1, 1)] \\

\midrule
\multirow{6}{*}{Lights} & Lighting Volume & volume & a set of lighting volume conditions \\
\cline{2-4}
 & Light Type  & light type & a set of light types \\
\cline{2-4}
 & \multirow{2}{*}{Light Position } & XZ position & Cartesian[Uniform(-20, 20), 0, Uniform(-20, 20)] \\
 &  & height & Uniform(5, 10) \\
\cline{2-4}
 & Light Intensity  & intensity range & Uniform(0.5, 3) \\
\cline{2-4}
 & Light Rotation  & orientation range & Face at Cartesian[Uniform(-50, 50), 0 Uniform(-50, 50)] \\

\midrule
\multirow{4}{*}{Multi-Group} & Group Number  & group number range & UniformRange(1, MaxNumGroups) \\
\cline{2-4}
 & Group Selection  & group activity & a set of modular groups \\
\cline{2-4}
 & \multirow{2}{*}{Group Placement } & group position & Cartesian[Uniform(-20, 20), 0, Uniform(-20, 20)]
 \\
 &  & group rotation & Euler[0, Uniform(0, 360), 0] \\
 
\midrule
\multirow{14}{*}{\shortstack{Activity\\Authoring}} & Character Number  & character number range & UniformRange(1, MaxNumCharacters) \\
\cline{2-4}
 & Multi-person Subgroup  & multi-person number range & UniformRange(0, MaxNum) \\
\cline{2-4}
 & Character Selection  & character & a set of 2200 characters \\
\cline{2-4}
 & \multirow{2}{*}{Character Texture } & body color & RGBA[Uniform(0.4, 1), Uniform(0.4, 1), Uniform(0.4, 1), Uniform(0.6, 1)] \\
 &  & clothes colors & HSV[Uniform(0, 1), Uniform(0, 1), Uniform(0.4, 1)] \\
\cline{2-4}
 & Character Alignment  & alignment method & a set of aligment methods \\
\cline{2-4}
 & Character Interval  & interval & Uniform(MinInterval, MaxInterval) \\
\cline{2-4}
 & \multirow{2}{*}{Character Perturbation } & position perturbation & Uniform(-0.25*interval, 0.25*interval)  \\
 &  & rotation perturbation & Uniform(-45$^{\circ}$, 45$^{\circ}$) \\
\cline{2-4}
 & Atomic Action  & atomic action & a set of permitted atomic actions \\
\cline{2-4}
 & \multirow{4}{*}{Animation } & animation clip & a set of animation clips \\
 &  & blended parameter & Uniform(0, 1) \\
 &  & speed & Uniform(0.8, 1.2) \\
 &  & normalized starting time & Uniform(0, 1) \\

\bottomrule
\end{tabular}
\end{center}
\vspace{-10pt}
\caption{List of randomizers, variables, and distributions used in  {\datagenerator}.}
 \vspace{-10pt}
\label{tab:domain_randomization}
\end{table*}

\subsection*{A.2. List of Variables for Domain Randomization}
\textit{Domain Randomization} allows {\datagenerator} to generate massive-scale diverse group activity data. 
Compared to PeopleSansPeople~\cite{ebadi2021peoplesanspeople},~{\datagenerator} contains a much higher degree of domain randomization for animating human motions and activities.
{\datagenerator} consists of a total of 14 atomic action classes and 384 animation clips, each with several blended style parameters such as character arm-space and stride. 
The domain randomization covers the scenes, cameras, lights, multi-groups, and activity authoring, as listed in Tab.~\ref{tab:domain_randomization}. We describe the randomizers in {\datagenerator} below.

\begin{algorithm}[t]
\caption{Dynamic speed adjustment for collision avoidance.}\label{alg:collision_avoidance}
\begin{algorithmic}[1]
\Require a list of instantiated characters and their initial animation speeds. 
\State At every frame,
\For{\textit{character} in Characters}
    \State \textit{init\_speed} $\gets$ Initial Speed of \textit{character}
    \State \textit{Speed} $\gets$ Current Speed of \textit{character}
    \State \textit{pos} $\gets$ Position of \textit{character} 
    \State \textit{forward} $\gets$ Forward Vector of \textit{character} 

    \State \textit{flag} $\gets$ False
    \For{\textit{other\_character} in Characters}
        \If{\textit{character} is not \textit{other\_character}}
            \State \textit{pos\_other} $\gets$ Position of \textit{other\_character} 
            \State \textit{offset} $\gets$ \textit{pos\_other} - \textit{pos}
            \State \textit{angle} $\gets$ Angle Between \textit{forward} and \textit{offset}
            \State \textit{dist} $\gets$ Length of \textit{offset}

            \If{\textit{dist} $\leq$ 0.8 $\And$ \textit{angle} $\leq$ 60}
                \State \textit{flag} $\gets$ True
            \EndIf
        \EndIf
    \EndFor
    \If{\textit{flag}}
            \State\textit{Speed} $\gets$ Max(\textit{Speed} * 0.96, 0.1) 
        \Else
            \State \textit{Speed} $\gets$ Min(\textit{Speed} * 1.03, \textit{init\_speed}) 

    \EndIf
\EndFor

\end{algorithmic}
\end{algorithm}

\begin{itemize}
\setlength\itemsep{-2pt}
\item \textbf{Scene Selection Randomizer} randomizes the selection of 3D scene.

\item  \textbf{HDRI Randomizer} randomizes the selection of panorama HDRIs.

\item  \textbf{Camera Position Randomizer} includes the randomizations of camera height, distance, and angle in a cylindrical coordinate.

\item  \textbf{Light Type Randomizer} randomizes the light type.
% the type of lights.

\item  \textbf{Light Position Randomizer} randomizes the positions of all lights. 

\item  \textbf{Light Intensity Randomizer} randomizes the intensities of all lights.

\item  \textbf{Light Rotation Randomizer} randomizes the rotations of all lights.

\item  \textbf{Group Number Randomizer} randomizes the number of groups being instantiated during the simulation.

\item  \textbf{Group Selection Randomizer} randomizes the selection of the activity for each group in the scene.

\item  \textbf{Group Placement Randomizer} randomizes the center position for each group.

\item  \textbf{Character Number Randomizer} randomizes the number of characters being instantiated in a group.

\item  \textbf{Multi-person Subgroup Randomizer} randomizes the number of 
% multi-person 
\textit{subgroups} in an activity, such as two persons talking to each other in a queueing group. This randomizer 
% only
applies to queueing and waiting groups.

\item  \textbf{Character Selection Randomizer} randomizes the selection of characters.

\item  \textbf{Character Texture Randomizer} randomizes the clothes and body colors of all characters.

\item  \textbf{Character Alignment Randomizer}  randomizes the method used to align characters in a group.

\item \textbf{Character Interval Randomizer} randomizes the interval between characters.

\item \textbf{Character Perturbation Randomizer} adds small perturbations to the characters' positions and rotations.

\item  \textbf{Atomic Action Randomizer}  randomizes the selection of permitted atomic actions.

\item  \textbf{Animation Randomizer} includes the randomization of animation clips, blended style parameters, animation speeds, and playback offsets.
\end{itemize}

%%%%%%%%%%%%%% Dataset
\section*{B. Datasets}
\noindent \textbf{\texttt{{\datagenerator}RGB}} contains 9K videos of multi-group and 6K videos of single-group activities, with a total of 6M RGB images and 48M bounding boxes. 
We show a collage of images from \texttt{{\datagenerator}RGB} in Fig.~\ref{fig:m3actrgb_images}, which contains diverse and realistic multi-group and single-group activities. 
(See our supplementary video for animated data samples.)
The distribution of \texttt{{\datagenerator}RGB} is also shown in Fig.~\ref{fig:m3actrgb_distr}. \texttt{{\datagenerator}RGB} contains as many as 19 persons per frame and an average of 8.1 persons per frame. 
Additionally, we show the comparison of several tracking datasets in Tab.~\ref{tab:tracking_dataset_comparison}. 
Even though we only selected the ``WalkRun'' and ``Dance'' data from \texttt{{\datagenerator}RGB} for the tracking experiments, the dataset size is much larger compared to MOT17~\cite{milan2016mot16} and DanceTrack~\cite{sun2022dancetrack}. 
In terms of the average number of tracks per video, our dataset is closer to DanceTrack. MOT17 mostly contains crowded scenes, while DanceTrack has only one dancing group per video.

\begin{table}[!t] 
\setlength{\tabcolsep}{2.5pt}
\small
  \aboverulesep=0ex
  \belowrulesep=0ex 
\begin{center}
\begin{tabular}{l|l|l|l}
\toprule
 Dataset & MOT17 \cite{milan2016mot16} & DanceTrack \cite{sun2022dancetrack} & \texttt{{\datagenerator}RGB}$^{\dag}$ \\
\midrule
 \#Videos & 14 & 100 & \textbf{2500} \\
 Avg. \#Tracks & \textbf{56} & 9 & 8 \\
 Avg. Track Len. (s) & 35.4 & \textbf{52.9} & 4.7 \\
 FPS (s) & 30 & 20 & 20 \\
 Total Frames & 11,235 & 105,855 & \textbf{250,000} \\
\bottomrule
\end{tabular}
\end{center}
\vspace{-10pt}
\caption{Comparison of multi-object tracking datasets. \texttt{{\datagenerator}RGB}$^{\dag}$ consists of ``WalkRun'' and ``Dance'' data used in our tracking experiments.}
\label{tab:tracking_dataset_comparison}
\end{table}

% \noindent \textbf{\texttt{{\datagenerator}2D}} was selected from a subset of single-group activities from \texttt{{\datagenerator}RGB} for 2D skeleton-based group activity recognition experiments, with all the semantic groups equally sampled.
% It contains a total of 10K videos and over 600K frames.
% In Fig.~\ref{fig:m3act2d_distr}, we plot the data distributions of \texttt{{\datagenerator}2D}. 

\noindent \textbf{\texttt{{\datagenerator}3D}} has 65K simulations of 3D single-group motions with a total duration of 87.6 hours, captured in 30 FPS.
Unlike \texttt{{\datagenerator}RGB} which contains equally simulated group activities, \texttt{{\datagenerator}3D} has different data sizes of all semantic groups based on their complexity.
The complexity of a group includes its alignment methods, permitted atomic actions, animation clips, and styles.
Fig.~\ref{fig:m3act3d_distr} shows the distribution of \texttt{{\datagenerator}3D}. 
Specifically, \texttt{{\datagenerator}3D} has more queueing groups than talking groups because the persons can form various shapes and more atomic actions can be performed within a queueing group.
We also slightly increased the range of the number of persons in the group for \texttt{{\datagenerator}3D}. 
On average, it has 6.7 persons for every single group and a maximum of 27 persons.

\begin{figure}[t]
\centering
   \includegraphics[width=\linewidth]{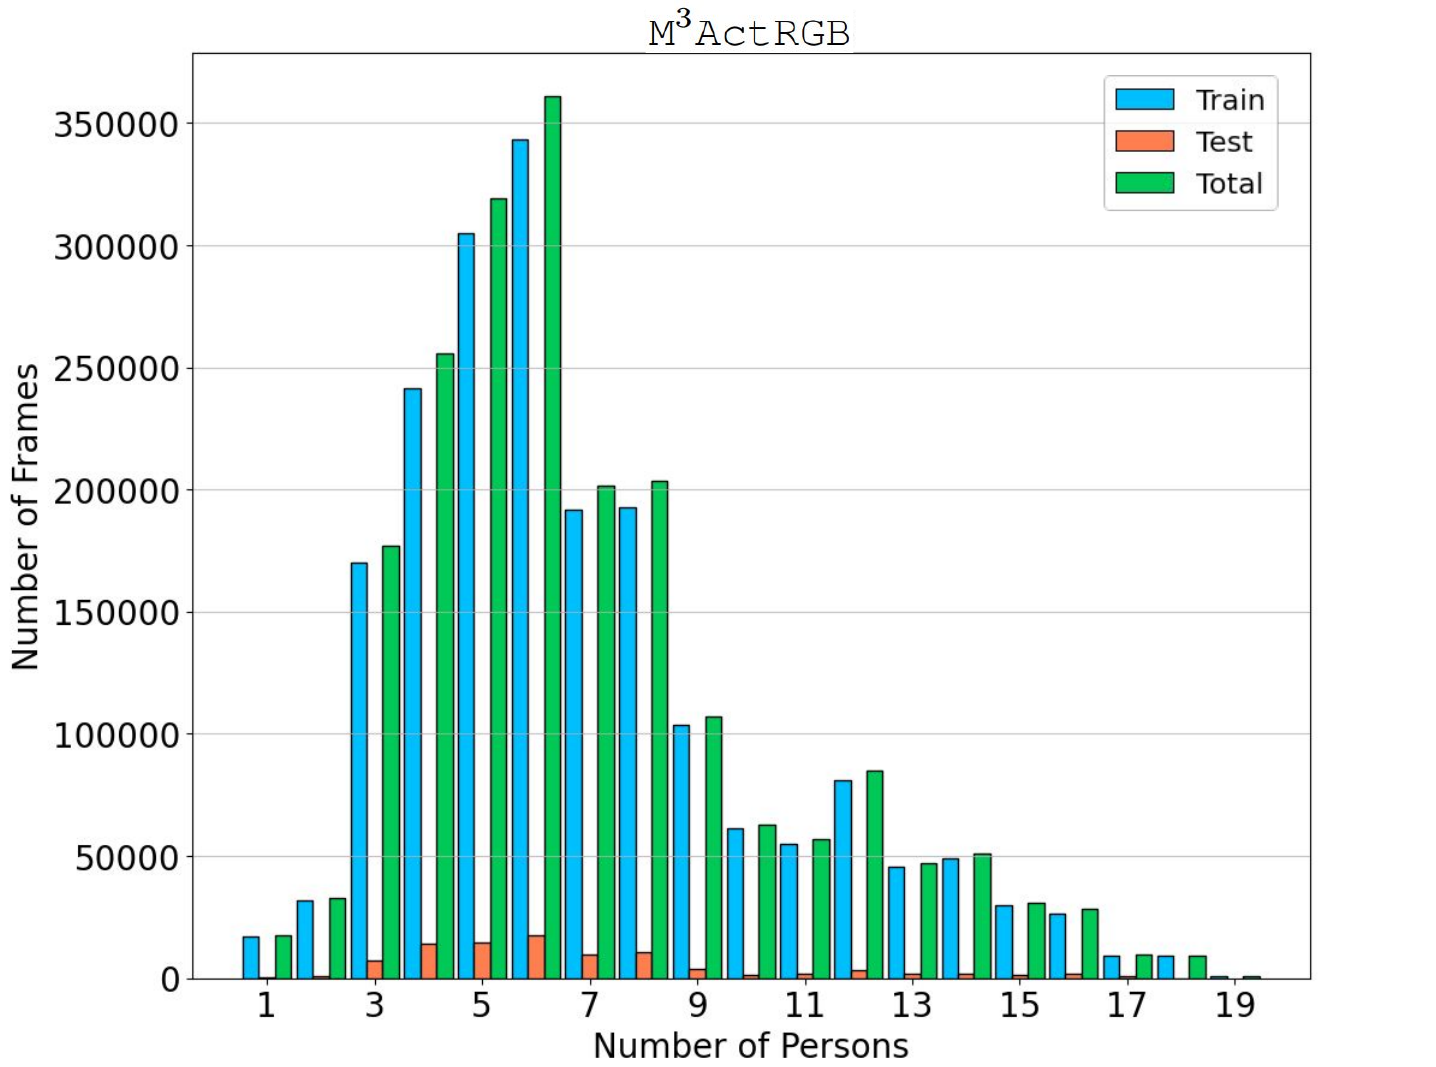}
   \caption{Distributions of \texttt{{\datagenerator}RGB}.}
\label{fig:m3actrgb_distr}
\end{figure}

% \begin{figure}[t]
% \centering
%    \includegraphics[width=\linewidth]{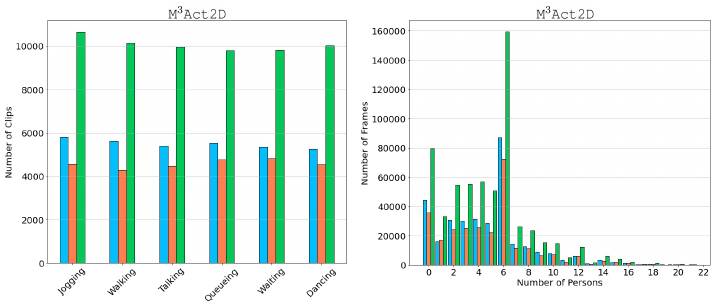}
%    \caption{Distributions of \texttt{{\datagenerator}2D} used for 2D skeleton-based group activity recognition.}
% \label{fig:m3act2d_distr}
% \end{figure}

\begin{figure}[t]
\centering
   \includegraphics[width=\linewidth]{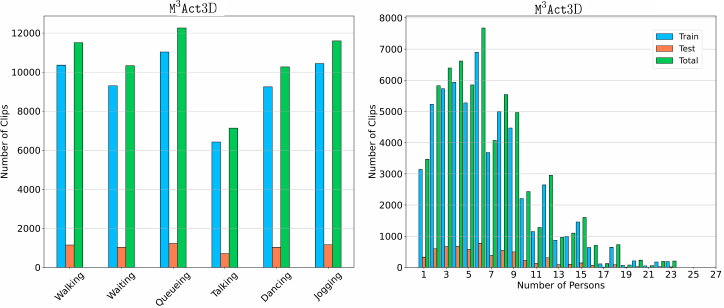}
   \caption{Distributions of \texttt{{\datagenerator}3D}.}
\label{fig:m3act3d_distr}
\end{figure}

%%%%%%%%%%%%%% Implementation Details
\section*{C. More Details of Experiments}
\subsection*{C.1 Multi-Person Tracking} 
The goal of multi-person tracking (MPT) is to predict the trajectories (bounding boxes + identification) of all persons across an image sequence from a dynamic video stream. 
Traditionally, multi-object tracking is approached by adding a re-identification layer, either using trainable architecture~\cite{wojke2017simple, Wojke2018deep} or applying heuristics-based algorithms~\cite{bewley2016simple}, on top of the object detection results, aiming to associate the bounding boxes across frames.
Recently, end-to-end methods~\cite{zeng2022motr, zhang2023motrv2} have shown to be more effective in several challenging datasets, such as DanceTrack~\cite{sun2022dancetrack} and MOT17~\cite{milan2016mot16}. 
To demonstrate the effectiveness of our synthetic data in enhancing real-world performance in multi-person tracking, we assess the impact primarily on MOTRv2~\cite{zhang2023motrv2}. 
It is an extension of MOTR~\cite{zeng2022motr} by incorporating YOLO-X~\cite{ge2021yolox} for bootstrapping detections. 
Using an end-to-end benchmark allows us to evaluate improvements with the synthetic dataset in both detection and identification.

\noindent \textbf{Implementation Details.}
We follow the same hyperparameters and data preprocessing procedure from the author-provided MOTRv2 repository\footnote{\url{https://github.com/megvii-research/MOTRv2}} for all training jobs. 
For mixed training with our synthetic data, we simply combined both data from \texttt{{\datagenerator}RGB} and DanceTrack as one large dataset, without any additional probability sampling from the real and synthetic data.
All models were trained with 16 NVIDIA A4000 GPUs, using a batch size of 1. 
It took roughly 7 days of training for all synthetic and real data combined.

\subsection*{C.2 Group Activity Recognition}
% \noindent \textbf{Formal Problem Formulation.}
% Group Activity Recognition (GAR) is a prominent computer vision task that detects the activity collectively performed by a group of actors 
% % interacting with one other 
% in a short video clip~\cite{wu2021comprehensive}. 
% Our {\datagenerator} contributes to generating large-scale datasets about human group activities, and we therefore examine the effectiveness of {\datagenerator}
% for GAR in \red{Sec. 4.2} of the main paper.

\jerry{revise this paragraph so that it convers the modified experiments in the main paper.}
State-of-the-art methods for group activity recognition (GAR) leverage 2D skeletons as input due to the effectiveness and robustness gained from the less biased and more action-focused
% skeleton-based
representation~\cite{thilakarathne2022pose,zhou2022composer,perez2022skeleton,zappardino2021learning,zhai2022spatial,actortransformer}. 
Let $[s_1,\cdots, s_t]$ denote a video with $t$ frames and $n$ persons, each frame $s_i:=\{p_1, \cdots, p_n\}$ where $p_i:=[(x_1, y_1, c_1), \cdots, (x_j, y_j, c_j)]$. Here, $j$ represents the number of joints in a person's skeleton, and each three-tuple $(x_j, y_j, c_j)$ respectively denotes the $x$ and $y$ coordinates in the pixel space and the class $c$ of the joint.
respectively denotes the $x$, $y$ coordinates in the pixel space and the class $c$ of the joint. 
For the given input $[s_1,\cdots, s_t]$, the objective of 2D skeleton-based GAR is to output the class of the group activity performed by the dominant group among these $n$ persons and identify the action class of each individual in the video. 
Usually, the task assumes each video has one dominant group, as any outlier person does not contribute to the group.

\noindent \textbf{Implementation Details.}
Our implementations of Composer~\cite{zhou2022composer} and Actor Transformer~\cite{actortransformer} for the experiments are based on the open-sourced implementation and hyperparameter settings\footnote{\url{https://github.com/hongluzhou/composer}}.
The only modified hyperparameter is the batch size, from $384$ to $256$ due to our computation constraints with an NVIDIA RTX 3090 graphics card.
Both Composer and Actor Transformer are transformer~\cite{vaswani2017attention} based architectures.
Note that both architectures are slightly modified after synthetic pre-training, due to the differences between the synthetic and real datasets in the maximum number of persons in a clip and the number of atomic action classes.
Specifically, we set a different maximum sequence length to the transformer encoders of Composer and Actor Transformer and replaced the last layers (i.e., the group activity classifier and the person action classifier) with new classifiers to output the correct data shape for CAD2.
In order to automatically determine whether or not the model training has saturated, we further adopted early stopping by setting a maximum number of $500$ epochs with an early stopping patience of $50$ epochs. 
The results (i.e., the number of epochs required for model convergence) reported in \red{Tab. 5} of the main paper include the $50$ epochs of the patience stage.

\subsection*{C.3 Controllable 3D Group Activity Generation}
Let $G^{TP} = \{m^{in}\}_{i=1 \sim T, n = 1\sim P}$ be a group of human motions with a total of $T$ frames and $P$ persons. 
The 3D pose of each person is denoted as $m^{in} \in R^{j\times d}$, where $j$ is the number of joints of a person and $d$ is the joint's feature dimension. 
We concatenate the global root position and all joints' 6D rotations~\cite{zhou2019continuity} as the pose representation.
% the pose representation $m^{in}$ is a concatenation of the global root position and all joints' rotation features ($\in R^{25\times 6}$) using the 6d representation~\cite{zhou2019continuity}.
% The concatenation was enabled by assuming an additional fake joint having the global root position as the feature of that fake joint.
Therefore, $j = 26$ (with $25$ actual joints) and $d = 6$.
% We concatenate the global root position and the joint rotations as the final pose representation, with $j = 26$ and $d = 6$. 
The same representation is used as the input for 3D group activity recognition with Composer~\cite{zhou2022composer} and used as the ground truth during training for both MDM~\cite{tevet2022human} and MDM+IFormer baselines for 3D group activity generation. 

\begin{figure}[t]
\centering
   \includegraphics[width=0.78\linewidth]{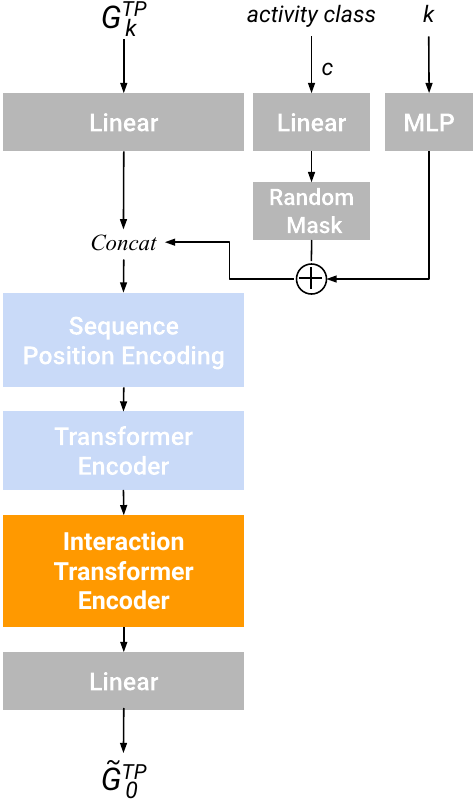}
   \caption{The architecture of MDM+IFormer. The model takes the
   noised
   % whole diffused 
   group motion $G^{TP}_k$, an activity class, and a time step $k$ as inputs and outputs $\tilde{G}^{TP}_0$, an estimation of the clean group motion.
   The interaction transformer encoder is ``added'' after the transformer encoder layer of MDM~\cite{tevet2022human} for modeling the person interactions.}
   \vspace{-15pt}
\label{fig:mdmiformer_architecture}
\end{figure}

\noindent \textbf{Composer for 3D Group Activity Recognition.}
% how do we get group/person latent feature extraction? What are the key hyperparams?
% \jerry{Honglu, we need your help to fill out this subsection.}
The learning-based metrics (recognition accuracy, FID, diversity, and multimodality)~\cite{guo2020action2motion} that are used to evaluate the generated 3D group activities require a well-trained 3D group activity \textit{recognition} model.
Composer~\cite{zhou2022composer} is a 2D skeleton-based group activity recognition model with a multi-scale transformer-based architecture. 
We chose Composer because it is a hierarchical architecture with fine-grained latent group-level and person-level features. 
We modified the first layer of Composer so that it accepts as input the aforementioned 3D group representation.
% same entire 3D 718 group motions 
We used the same set of hyperparameters as the GAR experiments including a learning rate of $0.0005$, a weight decay of $0.001$, a hidden dimension of $256$ for the transformer encoders, except a batch size of $64$, a maximum number of $27$ persons, and a total number of $26$ joints. 

After the 3D group activity recognition model is well-trained, 
we obtain the 3D group activity recognition accuracy, and extract
latent group and person features to calculate the FID, diversity, and multi-modality metrics.
The latent group representation is the learned CLS token from the \textit{last} block and last scale of the Multi-Scale Transformer module of Composer, whereas the latent person representations are the learned person tokens from the \textit{last} block and the second scale (i.e., the transformer encoder of the person scale) of the Multi-Scale Transformer module.

\noindent \textbf{MDM \& MDM+IFormer.}
% Formal equations used in MDM to describe the use of MDM+IFormer in GAG, including framework (with figure, hyperparams), loss, and sampling
We follow the same diffusion scheme as MDM~\cite{tevet2022human} to obtain the noised group activity at every $k$-th diffusion time step, $G^{TP}_k$. 
Specifically, $G^{TP}_0 := G^{TP}$, meaning no noise is added at the $0$-th diffusion time step. 
The reversed diffusion process is then formulated as: 
\begin{equation}
    \tilde{G}^{TP}_0 = D(G^{TP}_k, k, c),
\end{equation}
where $D$ is the MDM+IFormer network, illustrated in  Fig.~\ref{fig:mdmiformer_architecture}. 
$\tilde{G}^{TP}_0$ is the estimated clean group activity and $c$ is the one-hot activity label.
The loss function follows the
% simple 
objective in~\cite{ho2020denoising} and is defined as:
\begin{equation}
    L = \left|\left|G^{TP}_0 - \tilde{G}^{TP}_0\right|\right|^2.
\end{equation}
Our implementations of the MDM and MDM+IFormer baselines for 3D group activity generation are based on the author-released implementation of MDM\footnote{\url{https://github.com/GuyTevet/motion-diffusion-model}}
% We used a total number of diffusion time steps $1,000$.
without any hyperparameter tuning.
Both models were optimized using the same loss function described above and trained on an NVIDIA RTX 3090 graphics card for 320K iterations.

\begin{table}[t]
\setlength{\tabcolsep}{2.4pt}
\small
  \aboverulesep=0ex
  \belowrulesep=0ex 
    \begin{center}
    \begin{tabular}{l|c|c|c|c|c}
        \toprule
        Pretrain $\rightarrow$ Finetune & HOTA$\uparrow$ & DetA$\uparrow$ & AssA$\uparrow$ & IDF1$\uparrow$ & MOTA$\uparrow$ \\
        \midrule
        N/A $\rightarrow$ 100\% MOT17 & 56.3 & 51.9 & 62.1 & 66.6 & 56.1 \\
        \midrule
        Syn $\rightarrow$ 20\%  MOT17 & 51.7 & 48.0 & 56.3 & 62.1 & 54.4 \\
        Syn $\rightarrow$ 40\%  MOT17 & 57.4 & 54.3 & 61.5 & 69.3 & 61.3 \\
        Syn $\rightarrow$ 60\%  MOT17 & 59.7 & 57.1	& 63.0 & 70.0 &	62.9 \\
        Syn $\rightarrow$ 80\%  MOT17 & 60.6 & 58.1 & 63.8 & 73.0 & 67.1\\
        Syn $\rightarrow$ 100\% MOT17 & \textbf{63.7} & \textbf{61.6} & \textbf{66.9} & \textbf{74.7} & \textbf{68.7}\\
        \bottomrule
    \end{tabular}
    \end{center}
    \vspace{-10pt}
    \caption{Tracking results on MOT17 with different amounts of real data.}
    \label{tab:mot_result}   
\end{table}

\noindent \textbf{Formulas of Social Repulsive Forces}~\cite{helbing2000simulating}.
The three position-based metrics (in \red{Sec. 4.3.1} of the main paper) are formulated as follows.

\noindent \textit{-- Repulsive interaction force:} 
\begin{equation} \label{eq:interaction_force}
    \vec{f}_{ij}^{int} = A \cdot exp[(r_{i} + r_{j} - d_{ij})/B] \cdot \vec{n}_{ij}.
\end{equation}
$\vec{f}_{ij}^{int}$ is the interaction force of character $j$ applied to character $i$. $A$ and $B$ are constants ($A:=2,000$ and $B:=0.08$). $r_{i}$ and $r_{j}$ are the radius of the characters. $d_{ij}$ is the distance between the characters. $\vec{n}_{ij}$ is the unit vector pointing from character $j$ to character $i$.

\noindent \textit{-- Contact repulsive force:}
\begin{equation} \label{eq:interaction_force}
    \vec{f}_{ij}^{cont} = k \cdot max(0, r_{i}+r_{j}-d_{ij}) \cdot \vec{n}_{ij},
\end{equation}
where $k$ is a constant ($k:=120,000$). 

\noindent \textit{-- Total repulsive force:}
\begin{equation} \label{eq:interaction_force}
    \vec{f}_{ij}^{total} = \vec{f}_{ij}^{int} + \vec{f}_{ij}^{cont}.
\end{equation}
All constants follow the social force model proposed in~\cite{helbing2000simulating}.

\noindent  \textbf{Generated 3D Group Activities.} Please refer to our supplementary video for the rendered 3D group activities generated by MDM and MDM+IFormer.

\begin{table}[t]
\setlength{\tabcolsep}{2.1pt}

\small
  \aboverulesep=0ex
  \belowrulesep=0ex 
    \begin{center}
    \begin{tabular}{l|c|c|c|c|c}
        \toprule
        Training Data & HOTA$\uparrow$ & DetA$\uparrow$ & AssA$\uparrow$ & IDF1$\uparrow$ & MOTA$\uparrow$ \\
        \midrule
        \footnotesize{DT} & 68.8 & 82.5 & 57.4 & 70.3 & 90.8  \\
        \footnotesize{DT + Syn (D)} & 59.0 & 75.5 & 46.1 & 59.0 & 82.6 \\
        \footnotesize{DT + Syn (WR)} & 70.1 & 83.1 & 59.4 & 72.5 & 92.0 \\
        \footnotesize{DT + Syn (WR+D)} & \textbf{71.9} & \textbf{83.6} & \textbf{62.0} & \textbf{74.7} & \textbf{92.6} \\
        \midrule
        \footnotesize{DT + Syn (Single-group)}  & 65.1 & 80.2 & 55.8 & 66.7 & 89.1 \\
        \footnotesize{DT + Syn (Multi-group)}  & \textbf{73.5} & \textbf{83.9} & \textbf{64.7} & \textbf{75.8} & \textbf{93.0} \\
        \bottomrule
    \end{tabular}
    \end{center}
    \vspace{-10pt}
    \caption{MPT results on DanceTrack under different synthetic data distributions (eg. group types). We use all single-group and multi-group data for the last two rows.}
    \label{tab:synthetic_data_type}   
\end{table}

%%%%%%%%%%%%%% MOT Experiments

%%%%%%%%%%%%%% Additional Experiments
\section*{D. Additional Experiments}

\subsection*{Replacing Real Data}
In \red{Sec 4.1}, we demonstrate that incorporating our synthetic data results in tracking performance comparable to that of MOTRv2*, the same method trained with 62.5\% more real data and an ensemble of four models. 
While the comparison provides valuable insights, it is also interesting to know the amount of real data that is replaceable by our synthetic data under more controlled conditions.
To achieve this, we first train the model with 100\% real data as a comparison baseline.
Then we maintain a fixed amount of synthetic data while gradually decreasing the amount of real data used for training. 
This enables us to observe the changes in tracking performances as well as identify how much real data can be replaced by synthetic data.
% where the performance of models trained only with 100\% real data falls in between the performances obtained when varying the amount of real data.
We conduct the experiment on MOT17~\cite{milan2016mot16}. 
We apply synthetic pre-training followed by real data fine-tuning as the training protocol because MOT17 contains more object classes. 
We adopt the same MOTRv2 architecture, hyperparameters, and synthetic data (``WalkRun'' and ``Dance'') as the main MPT experiment. 
We pre-trained the model on synthetic data for 5 epochs and then fine-tuned it for 20 epochs for all conditions.

Tab.~\ref{tab:mot_result} presents the tracking results on MOT17~\cite{milan2016mot16}.
First, pretraining with our synthetic data leads to significant performance gain on all five metrics, compared to the model without pretraining.
Second, we see that the performance improves with the increased amount of real data. 
It's worth noting that the model trained on synthetic data and only 20\% (or less) real data is inferior to the same model trained on 100\% real data without pretraining, which suggests a domain gap between the synthetic and real data.
Last but most importantly, the model trained only on 100\% real data achieves comparable performance to the model trained on 20\% to 40\% of real data with synthetic pretraining.
This shows that \textit{our synthetic data is equivalent to 60\% to 80\% of MOT17 training data.}
In other words, our synthetic data can at least reduce 60\% of MOT17 data required for training.

\subsection*{Impact of Synthetic Data Distributions}
We investigate the influence of synthetic data distributions on downstream model performance. 
We present additional tracking results on DanceTrack, with various group types for training, detailed in Table \ref{tab:synthetic_data_type}. 
These results reveal that training with multi-group synthetic data, such as "WR" and "Multi-group," leads to superior performance. 
The high complexity inherent in multi-group settings, with frequent identity switches, proves advantageous for tracking individuals in dynamic movements on DanceTrack. 
Our findings suggest that \textit{synthetic datasets with apparent similarities in data complexity and distribution to target datasets tend to enhance model performance.} 
It also underscores the importance of having a flexible data generator, such as the modular and highly parameterized groups in {\datagenerator}, which facilitate parameter tuning and allow for the customization of synthetic data distributions to closely approximate those of downstream datasets.

\subsection*{Faster Convergence}
Pretraining with data from {\datagenerator} can improve convergence speed on the target dataset. We conduct the GAR experiment using 2D keypoints as the only input modality for both models and compare the number of epochs required for model convergence in Tab.~\ref{tab:convergence}. For example, training Composer from scratch on CAD2 requires 88 epochs on average; with \texttt{{\datagenerator}} pre-training, Composer only requires 13 epochs for convergence. 

\begin{table}[]
\small
  \aboverulesep=0ex
  \belowrulesep=0ex 
\begin{center}

\begin{tabular}{l|l|c}
\toprule
\multicolumn{2}{l|}{\textbf{\#Epochs required for model convergence}} & \textbf{Target}   \\ \cline{3-3}
\multicolumn{2}{c|}{(Composer~\cite{zhou2022composer} / Actor Transformer~\cite{actortransformer})}   & CAD2~\cite{choi2011learning}     \\ \midrule
\multirow{2}{*}{\textbf{Source}}                     & CAD2~\cite{choi2011learning}                     & 88 / 233 \\
                                            & \texttt{\datagenerator}                   & 13 / 92  \\ \bottomrule
\end{tabular}
\end{center}
\vspace{-10pt}
\caption{Pre-training with our synthetic data leads to faster model convergence on the target domain for GAR. (Composer: $6.8\times$ faster; Actor Transformer: $2.5\times$ faster) }
\label{tab:convergence}
\end{table}

%%%%%%%%%%%%%% Limitations and Future work
\section*{E. Limitations \& Future Work}
% \jerry{consider adding multi-group interactions, and navigation or interaction with environments/objects. Zero-shot transfer --- domain gaps still remain.}
We demonstrate that our synthetic data can replace a great amount of real data and successfully mitigate the scarcity of real data for multi-person and multi-group tasks, despite the domain gap that restricts the generalizability of models trained with synthetic data. 
With the release of our data generator, {\datagenerator}, we encourage the community to create their own data or enhance the synthetic data generator.
While collecting more assets and generating more data with adjusted camera views can surely increase data diversity and shorten the gap,
we would also like to point out some aspects of the generator that should be addressed in the future to create more realistic data.

\noindent \textbf{Publicly-available assets.}
Most assets we use in {\datagenerator} are publicly available, including HDRIs, human characters, and animations. 
However, most existing assets such as photometric 3D scenes and high-quality avatars may require additional licensing for model training. 
Some assets could be restricted to specific game engines, which hinders the development of synthetic data. 

\noindent \textbf{Simulated Hair and clothes.}
The avatars used in {\datagenerator} do not contain hair and clothes physics that are in accordance with their body motions. 
Adding cloth and strand-based hair simulation would be sufficient for realistic interactions between hair/cloth and body, and thus improve the data quality.

\noindent \textbf{Finger and face Movements.}
Our animations do not contain finger and face movements. 
While it might be reasonable as human groups are generally captured from a distance, adding finger and face movements can still improve the fidelity of the human motions.

\noindent \textbf{Human-environment interactions.}
Like most synthetic datasets \cite{black2023bedlam, yang2023synbody, varol2017learning, bazavan2021hspace}, {\datagenerator} lacks meaningful interactions between human and environment. 
The interactions might include groups of humans navigating in a complex environment, a person picking up a phone while texting, or holding a suitcase.
Animating human motions and activities with scene awareness is incredibly challenging. 
A simple solution is to polish each scene by carefully placing the avatars and staging the human behaviors. However, it would require significant manual efforts and limit the scale and diversity of the synthetic data.

\noindent \textbf{Complexity for human groups.}
Animating human groups is significantly more challenging than animating the motions of a single person because the complexity (the number of interactions) increases quadratically as the number of persons increases.
We apply relatively simple heuristics when designing rules for authoring human groups, which could only reflect a certain portion of real-world activities. 
These underlying rules that drive the group motions could also lead to datasets that are less complex than real-world ones, limiting the model generalization on downstream tasks.
Creating new groups with expert-guided heuristics, LLM-generated rules, or directly from the 3D GAG method, should be considered.
An alternative would be using existing motion capture data in replace of the procedural generation method. 
However, the lack of fine-grained motion capture data for large-scale collective 3D group motions is an obstacle to the development.

\noindent \textbf{Societal Impacts.}
While we demonstrate the effectiveness of our synthetic data on several tasks, it is important to note that the use of synthetic data, in all manners, may still result in unbalanced and biased results.
We strive to ensure the inclusiveness and fairness of our datasets by incorporating human avatars of all ages, genders, and ethnicities, providing a representative and equitable approach to generating data for responsible advancement in related fields.

\begin{figure*}[t]
\centering
   \includegraphics[width=\linewidth]{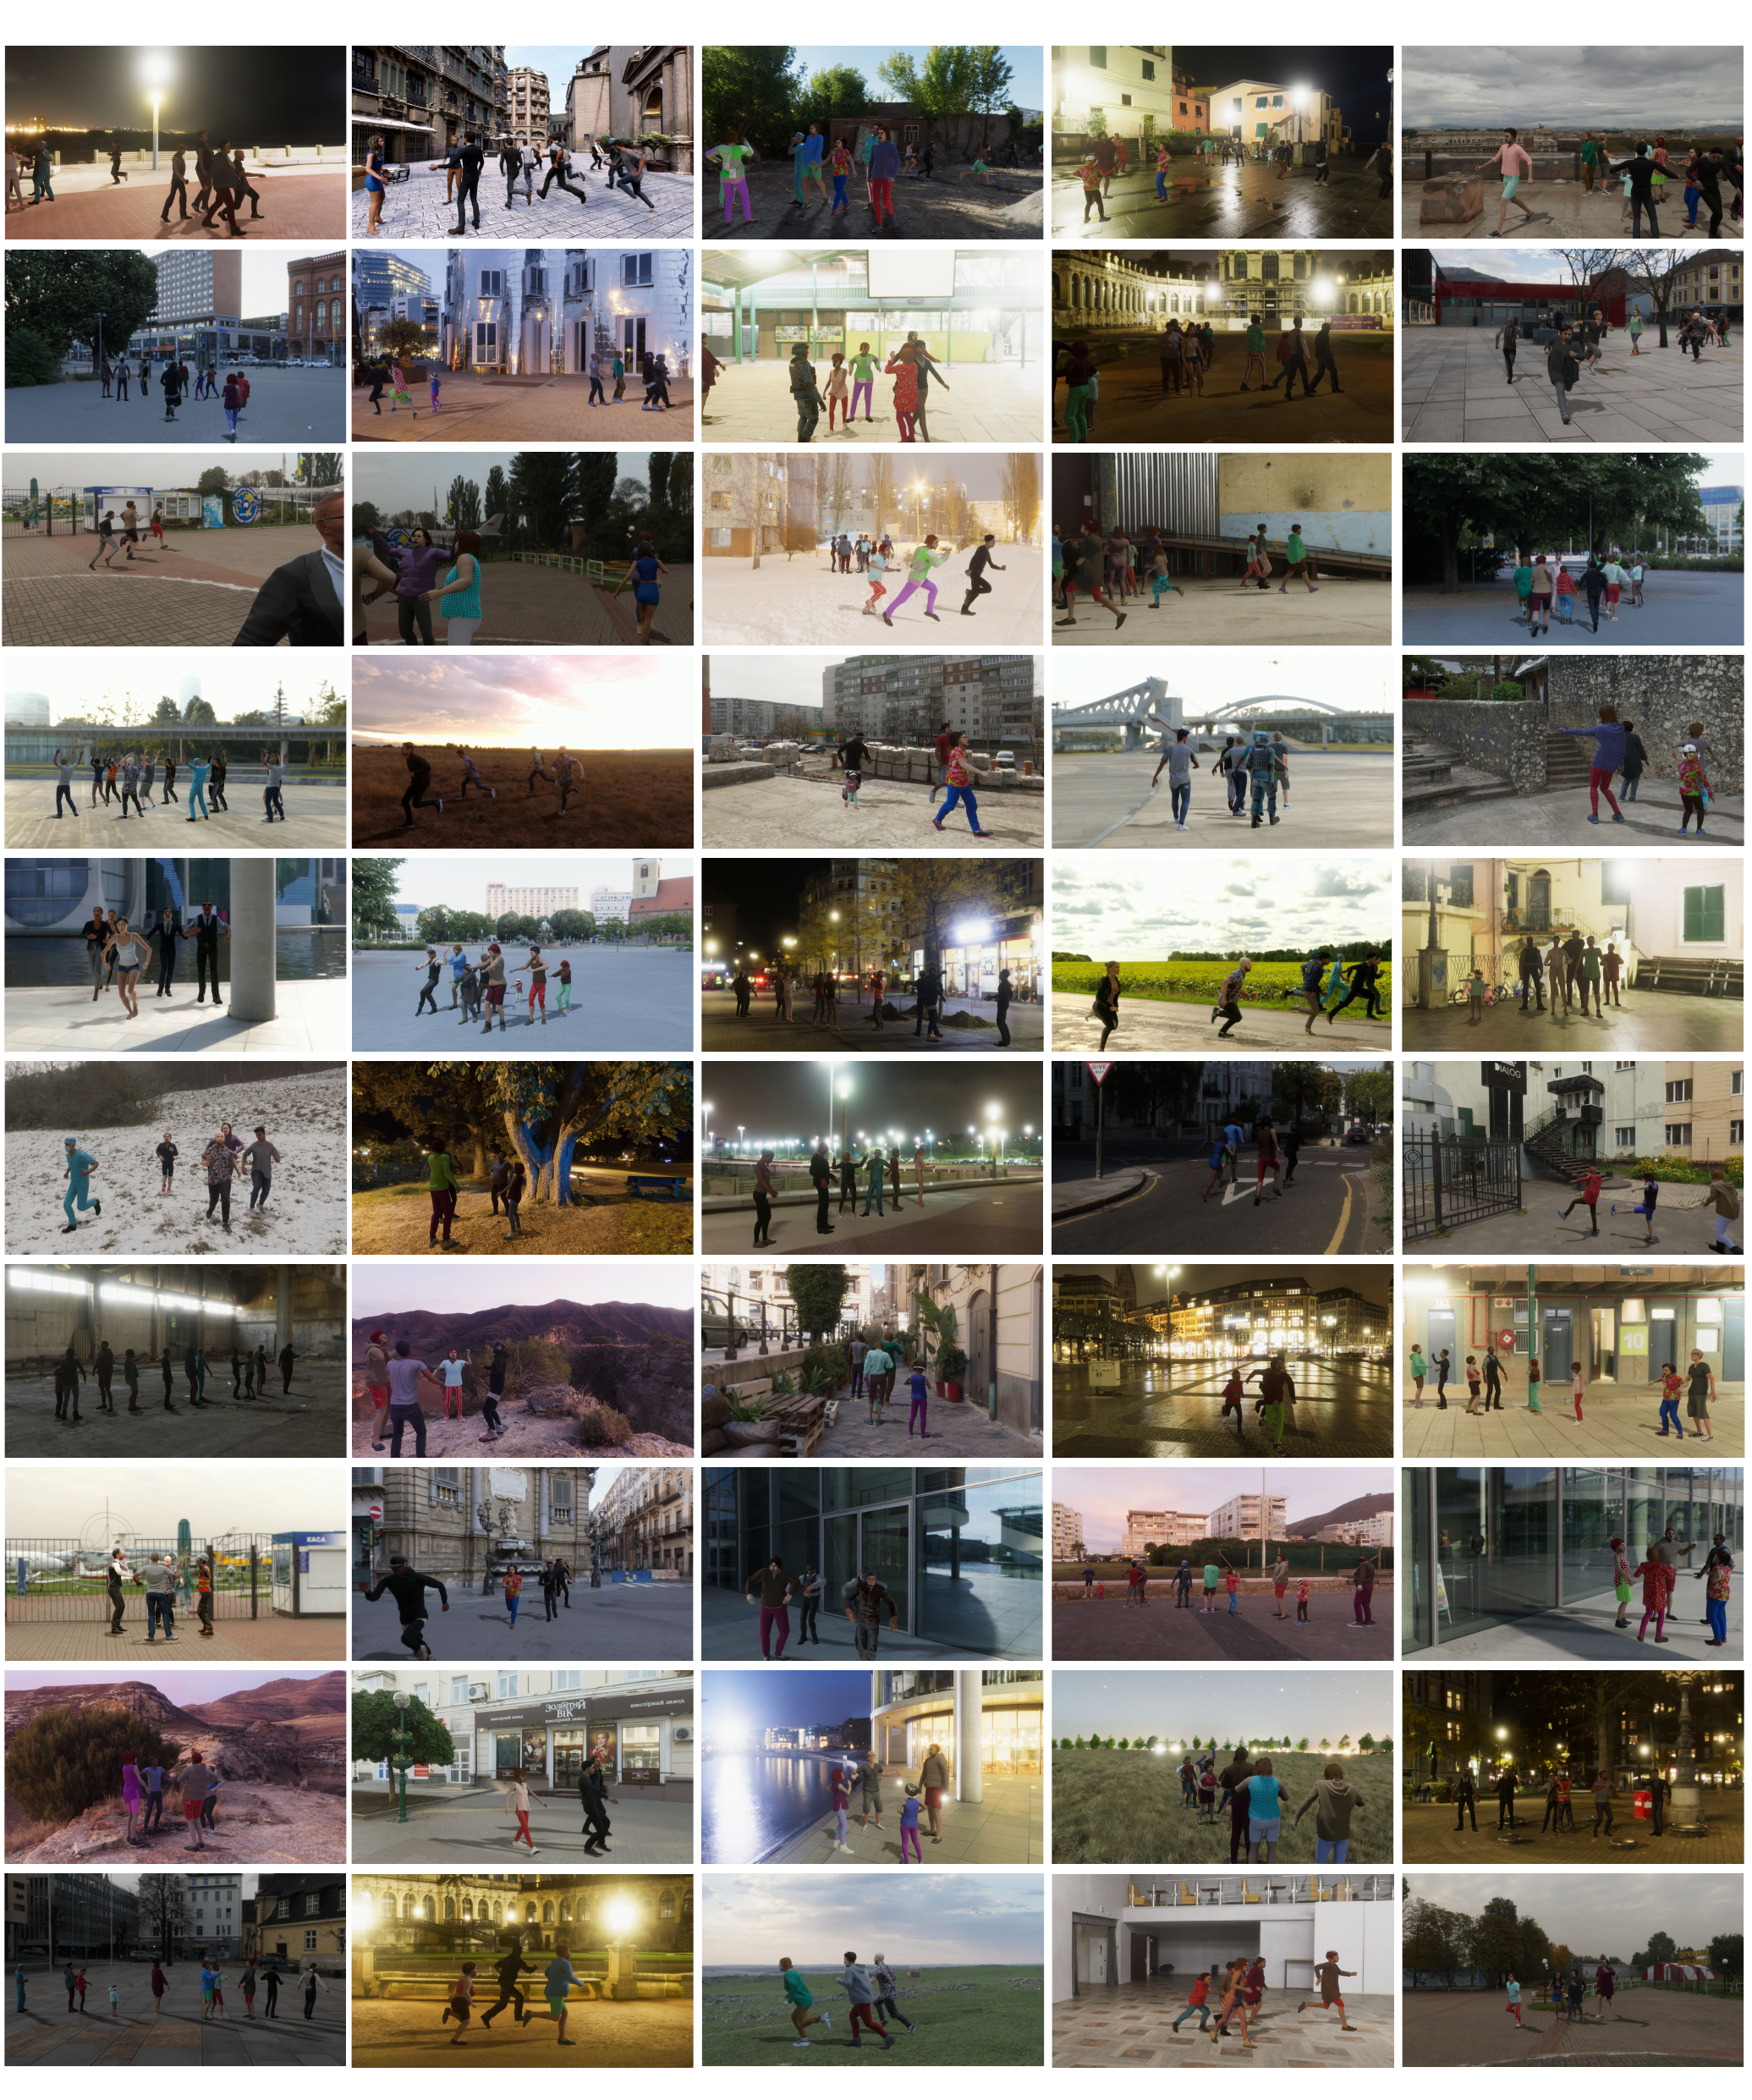}
   \caption{Collage of images from \texttt{{\datagenerator}RGB}, including multi-group activities (first 3 rows) and single-group activities (last 7 rows).}
\label{fig:m3actrgb_images}
\end{figure*}

% \newpage
